# Supplementary material for: Motion Forecasting via Model-Based Risk Minimization
Source: arXiv:2409.10585 source file (2024-09-20)
Supplement: Supplementary file 1 [file appendix.tex]

\section*{APPENDIX}
\label{app:nms}
Below, we visualize the numerical values for NMS+KMeans as a function of the threshold as an extension of Tab. \ref{tab:benchmark_sampling_methods}. 
In \ac{NMS}, we first select the trajectory with the highest probability and remove it from the set. Next, we eliminate all trajectories with an \ac{ADE} below a certain threshold relative to the selected trajectory. This process is repeated until $k$ trajectories are selected. 
Overall, we observe a strong dependence of the performance on the threshold value. We find the best threshold value to be 1.
\begin{figure}[h]
\begin{center}
\includegraphics[width=1\linewidth]{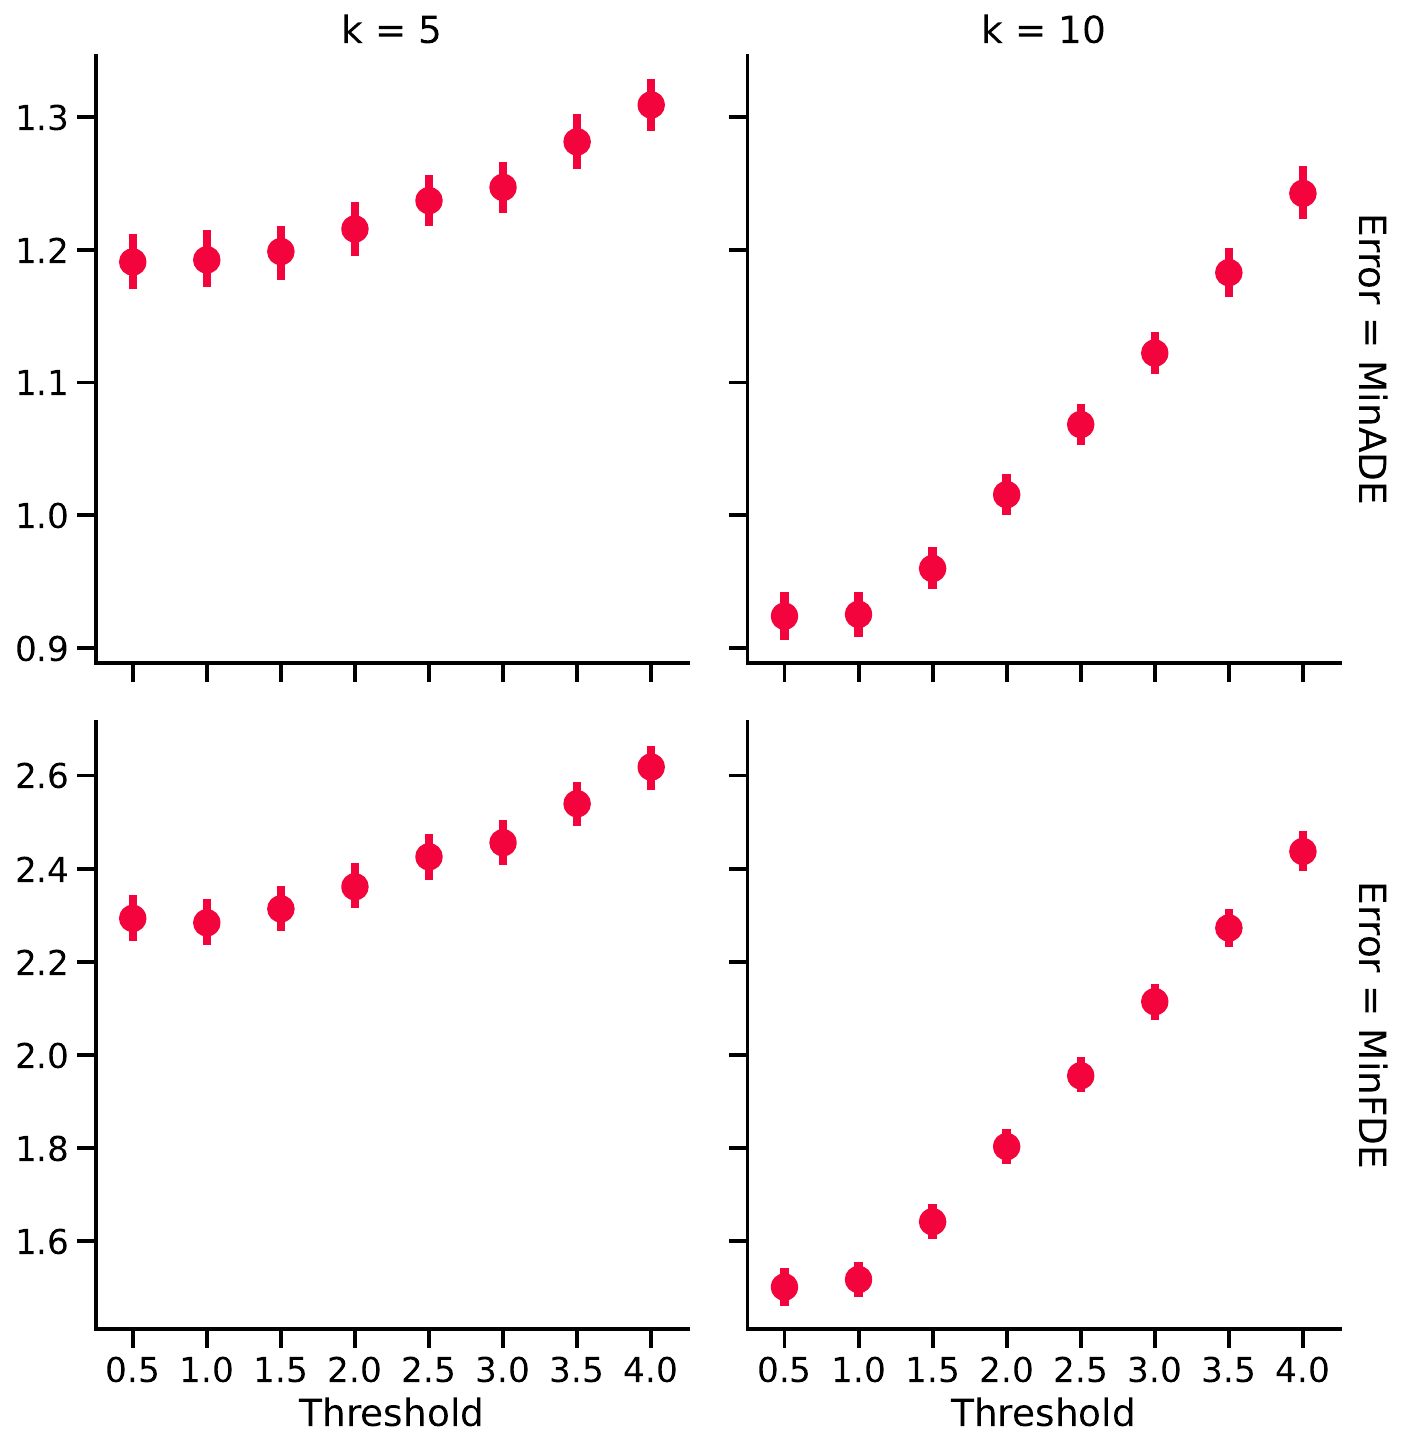}
\end{center}
\caption{Change of the $\text{\ac{minFDE}}_k$ and $\text{\ac{minADE}}_k$ for different $k$ values as a function of the threshold for NMS+KMeans. }
\label{fig:nms_study}
\end{figure}
%\section*{ACKNOWLEDGMENT}
%Put sponsor acknowledgments in the unnumbered footnote on the first page.
